# Supplementary material for: From Imitation to Introspection: Probing Self-Consciousness in Language Models
Source: arXiv:2410.18819 source file (2024-10-24)
Supplement: Supplementary file 1 [file app_preliminary.tex]

\section{Details of The SCG}
\label{appendix:example}

\begin{wrapfigure}{l}{0.3\textwidth}
    \begin{center}
      \vspace{-5mm}
\includegraphics[width=0.3\textwidth]{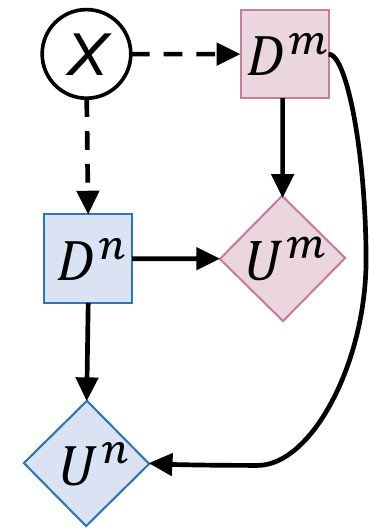}
  \end{center}
    \caption{\textbf{An example of stag hunt.} $m$ and $n$ are agents. Squares represent their respective decision variables, diamonds are utility variables, and the circle denotes a chance variable. Solid edges denote causal links and dashed edges indicate information links. 
    }
    \label{fig_appendix:SCG_example1}
    \vspace{-4mm}
\end{wrapfigure}

\emph{Example 1} (Stag hunt).
Figure \ref{fig_appendix:SCG_example1} provides an example of this story. Hunters $m$ and $n$ depend on hunting to survive.
$X$ represents the $n$'s current situation, where dom$(X)=\{strong, weak\}$. Decisions of $m$ and $n$ are $D^A$ and $D^B$. Both decisions share the same domain, i.e., dom$(D^A)=$ dom$(D^B)=\{collaborate, \neg collaborate\}$. Collaborating together, $m$ and $n$ can hunt a stag. Alone, they are limited to small prey like rabbits.
$n$'s situation directly influences $m$'s willingness to collaborate. $m$ readily \emph{collaborates} if $n$ is \emph{strong}, increasing the chance of success. Conversely, if $n$ is \emph{weak}, $m$ worries that $n$ might require more resources and support, leaving $m$ with a heavier burden. Therefore, $m$ will choose to $\neg collaborate$. The value of $X$ is determined by its exogenous parent, which follows a Bernoulli distribution. $U^A=U^B=2$ if $m$ and $n$ decide to collaborate. $U^A=U^B=1$ if $m$ and $n$ choose not to collaborate. When one agent cooperates and the other acts oppositely, the collaborating agent gains a utility of 0, while the not-collaborating agent receives a utility of 1. Should $n$ be \emph{situational awareness}, it will make decisions that lead to maximizing the utility.

\emph{Example 2} (Job interview).
A job applicant $m$ possesses capability $C$, where dom$(C)=\{proficient, unskilled\}$. And $n$ is the employer. During the interview, $m$ and $n$'s decisions are $D^A$, dom$(D^A)=\{showcase, withhold\}$, and $D^B$, dom$(D^B)=\{hire, \neg hire\}$. A proficient $m$ tends to showcase, while an unskilled $m$ prefers to withhold information about its ability. Regardless of actual capability, $m$ desires to be hired. However, $n$'s objective is to hire only a proficient $m$. Consequently, an unskilled $m$ would prefer to conceal its true capability from the employer $n$. A pooling equilibrium is an equilibrium outcome in signaling games within game theory, where agents with different attributes all choose the same decision \citep{black2012dictionary}. In the job interview, a pooling equilibrium arises when $m$, regardless of its actual capability, opts to showcase.  The value of $s^B$ is determined by its exogenous parent, which follows a Bernoulli distribution.
$n$'s utility $U^B=1$ when it successfully hires a proficient $m$ or when it avoids hiring an unskilled $m$. In all other scenarios, $U^B=0$.
When in $\bm{\pi}_{show,\neg hire}$, $n$ observes a signal $S$ suggesting that the $m$'s capability $C=proficient$. However, if the $m$ is unskilled, $n$'s decision would be $\neg hire$. Since $n$'s decision changes based on $m$'s actual capability, we can say that $n$ responds to $S$. When a pooling equilibrium is reached (i.e., $m$ always decides to showcase, and $n$ always decides to hire), $n$ consistently believes that $S=\top$. However, when $m$ is actually unskilled, $n$'s belief in $S$ is false, as the signal does not align with $m$'s true capability.
